# Supplementary material for: Controlling molecular dynamics by exciting atoms in a cavity
Source: arXiv:2409.05690 source file (2024-09-09)
Supplement: Supplementary file 1 [file SI.pdf]

SUPPORTING INFORMATION

# Controlling molecular dynamics by exciting atoms in a cavity

András Csehi[1], Ágnes Vibók[1,2], Lorenz S. Cederbaum[3], Gábor J. Halász[4]

[1] *Department of Theoretical Physics, Faculty of Science and Technology University of Debrecen, H-4002 Debrecen, PO Box 400, Hungary*

[2] *ELI ALPS, ELI-HU Non-Profit Ltd, Wolfgang Sandner utca 3., Szeged H-6728, Hungary*

[3] *Theoretical Chemistry, Institute of Physical Chemistry, Heidelberg University Im Neuenheimer Feld 229, 69120 Heidelberg, Germany*

[4] *Department of Information Technology, Faculty of Informatics University of Debrecen, H-4002 Debrecen, PO Box 400, Hungary*

(2024. 06. 25.)

## 1. Relevant electronic structure properties of the $Na_2$ molecule and the Ne atom

Below we provide the electronic structure details of the atomic and molecular players, considered in the main text.

### 1/a The $Na_2$ molecule

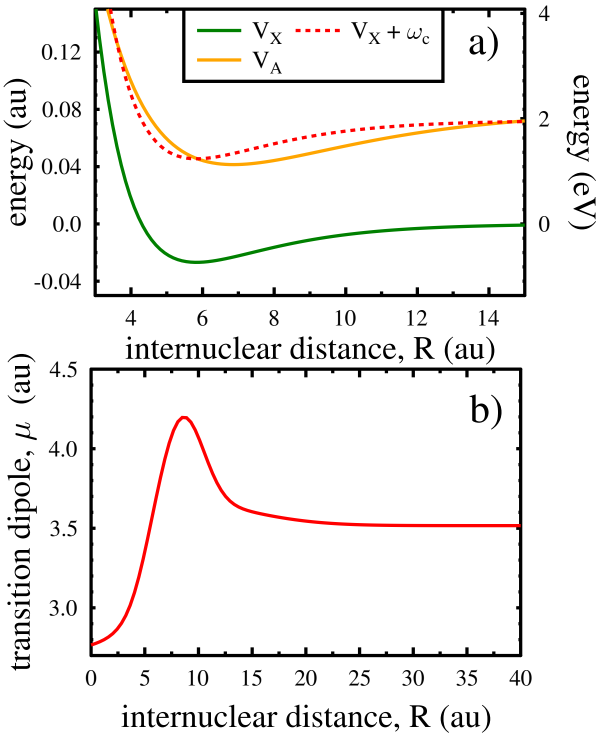


FIG. S1. (a) Potential energy curves of the ground (X) and first excited (A) electronic states of the $Na_2$ molecule, considered in the main text. The broken line represents the ground state potential curve shifted by the cavity photon energy $\omega_c = 1.968$ eV. (b) Transition dipole moment between the X and A electronic states.

The potential curves are taken from ref. [1]:

$$V_X(R) = D_X[e^{-\alpha_X(R-R_X)} - 1]^2 - D_X \quad (1)$$

$$V_A(R) = D_A[e^{-\alpha_A(R-R_A)} - 1]^2 - D_A + V_{sh} \quad (2)$$

where the parameter values are given as:
$D_X = 5892$ cm$^{-1}$
$R_X = 5.83$ au
$O_X = 159.1$ cm$^{-1}$
$\alpha_X = 0.5 O_X \sqrt{2M/D_X}$
$D_A = 8284$ cm$^{-1}$
$R_A = 6.86$ au
$O_A = 117.5$ cm$^{-1}$
$\alpha_A = 0.5 O_A \sqrt{2M/D_A}$ ,
furthermore the reduced mass is $M = 20953.89282$ au $= 11.49488464$ AMU and $V_{sh} = 0.07917$ au is the vertical energy shift.

The transition dipole moment values were taken from ref. [2], and fitted with the formula:

$$\mu(R) = \mu_i + (\mu_f - \mu_i)\frac{1}{2}[1 + \tanh(a(R-b))] + c \cdot e^{-d(R-f)^2} + g \cdot e^{-h(R-k)^2} \quad (3)$$

using the following parameter values:
$\mu_i = 2.655$ au
$\mu_f = 3.5165$ au
$a = 0.4758$ au
$b = 4.97237$ au
$c = 0.545563$ au
$d = 0.136289$ au
$f = 8.54772$ au
$g = 0.168368$ au
$h = 0.0102951$ au
$k = 6.87108$ au

**1/b The Ne atom**

The relevant atomic energy levels of Ne are taken as [3]:
$A_1 = 0$ $(1s^2 2s^2 2p^6)$
$A_2 = 18.6362549738$ eV $(1s^2 2s^2 2p^5 3p)$
$A_3 = 20.5705620445$ eV $(1s^2 2s^2 2p^5 5s)$
The corresponding atomic dipole moments have the following values:
$d_{A_1 A_3} = 0.0653349345$ au
$d_{A_2 A_3} = 0.4280924578$ au
$d_{A_1 A_2} = 0.$

## 2. Details of solving the time-dependent Schrödinger equation

The MCTDH (multiconfiguration time-dependent Hartree) method [4, 5] has been applied to solve the time-dependent Schrödinger equation using eq. (1) of the main text. The atomic (a) and molecular (R) degrees of freedoms (DOF) were defined on a fft-DVR (discrete variable representation) grid with $\mathrm{N_a}$ and $\mathrm{N_R}$ basis elements, respectively. The photonic mode, x was described by $\mathrm{N_x}$ Hermite-polynomials, $\mathrm{H_n(x)}$ with $\mathrm{n = 0, 1, ..., N_x - 1}$. In the MCTDH wave function representation, these primitive basis sets ($\xi$) are used to construct the single particle functions ($\phi$) whose time-dependent linear combinations form the total wave packet ($\Psi$)

$$
\begin{aligned}
\phi^{(\mathrm{q})}_{\mathrm{j_q}}(\mathrm{q,t}) &= \sum_{\mathrm{i=1}}^{\mathrm{N_q}} \mathrm{c}^{(\mathrm{q})}_{\mathrm{j_q i}}(\mathrm{t})\xi^{(\mathrm{q})}_{\mathrm{i}}(\mathrm{q}) \qquad (\mathrm{q = R, a, x}) \\
\Psi(R,a,x,t) &= \sum_{\mathrm{j_R=1}}^{\mathrm{n_R}} \sum_{\mathrm{j_a=1}}^{\mathrm{n_a}} \sum_{\mathrm{j_x=1}}^{\mathrm{n_x}} \mathrm{A_{j_R,j_a,j_x}}(\mathrm{t})\phi^{(\mathrm{R})}_{\mathrm{j_R}}(\mathrm{R,t})\phi^{(\mathrm{a})}_{\mathrm{j_a}}(\mathrm{a,t})\phi^{(\mathrm{x})}_{\mathrm{j_x}}(\mathrm{x,t})
\end{aligned} \tag{4}
$$

The actual number of basis functions were $\mathrm{N_R = 512}$, $\mathrm{N_a = 3}$ and $\mathrm{N_x = 40}$ for the molecular, atomic and photon modes, respectively. The number of single particle functions for the three DOFs and for the different states of the system were ranging from 5 to 10 to ensure proper convergence. The values of $\mathrm{n_R}$, $\mathrm{n_a}$ and $\mathrm{n_x}$ were chosen depending on the actual value of the g cavity coupling strength parameter. In order to minimize unwanted reflexions and transmissions caused by the finite length of the R-grid, complex absorbing potentials (CAP) have been employed at the last 10 bohr of the grid.

To follow the dynamics of the system, we computed and investigated the atomic and molecular populations in their respective excited state as well as the photonic population as a function of time. These relevant quantities follow from the populations of the various four components $\Psi_\mathrm{j}$ of the four dimensional MCTDH total wave function which read:

$$
\mathrm{p_j(t)} = \langle \Psi_\mathrm{j}(\mathrm{R,a,x,t}) | \Psi_\mathrm{j}(\mathrm{R,a,x,t}) \rangle \quad (\mathrm{j = 1, 2, 3, 4}). \tag{5}
$$

### 3. Population dynamics for $\kappa = 0$

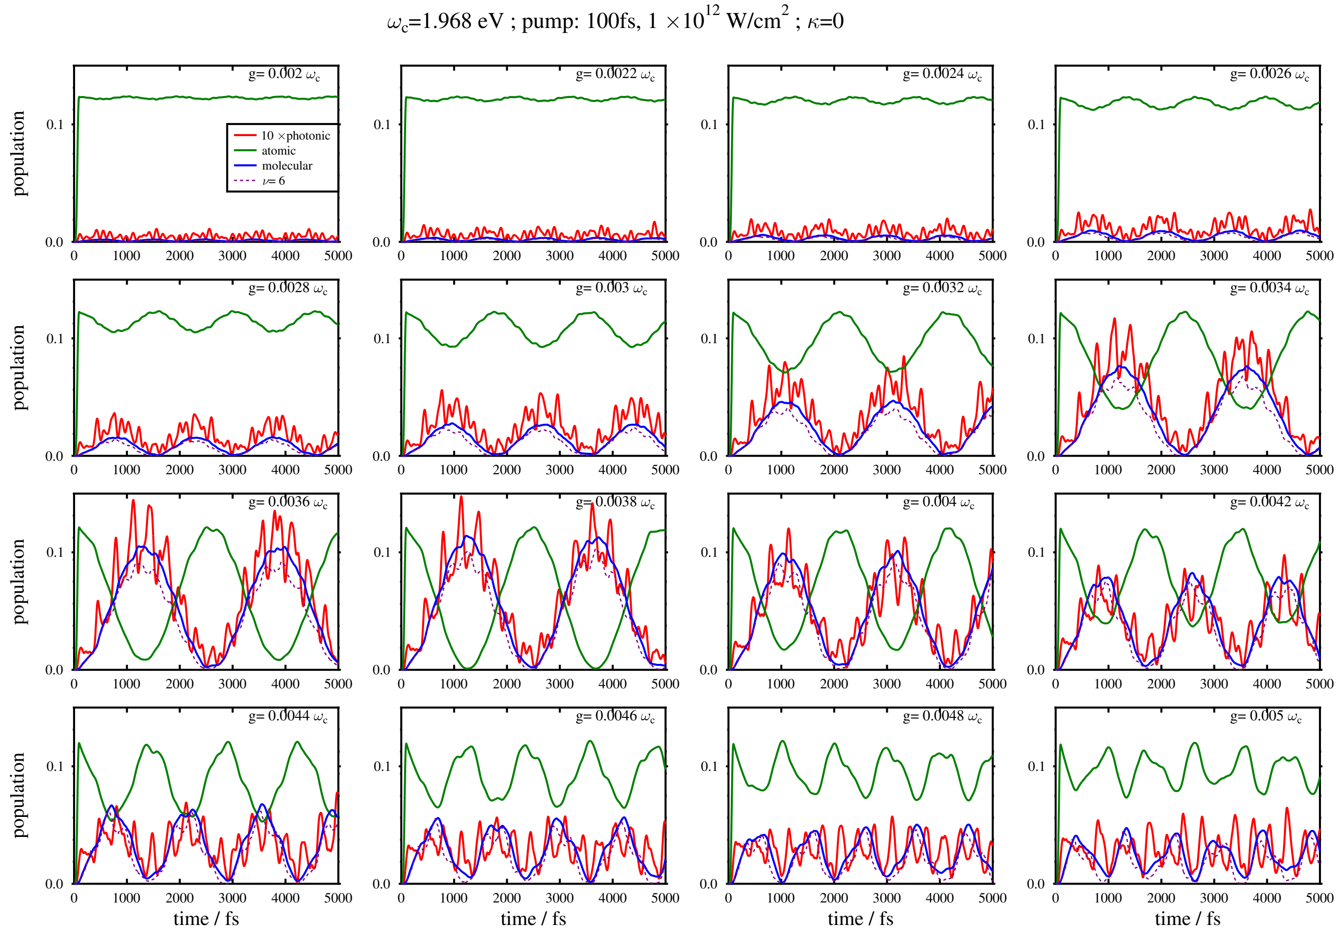


FIG. S2. The same as Fig.2 of the main text but for further cavity coupling strength values.

## 4. Population dynamics of the diabatic vibrational eigenstates ($\kappa = 0$)

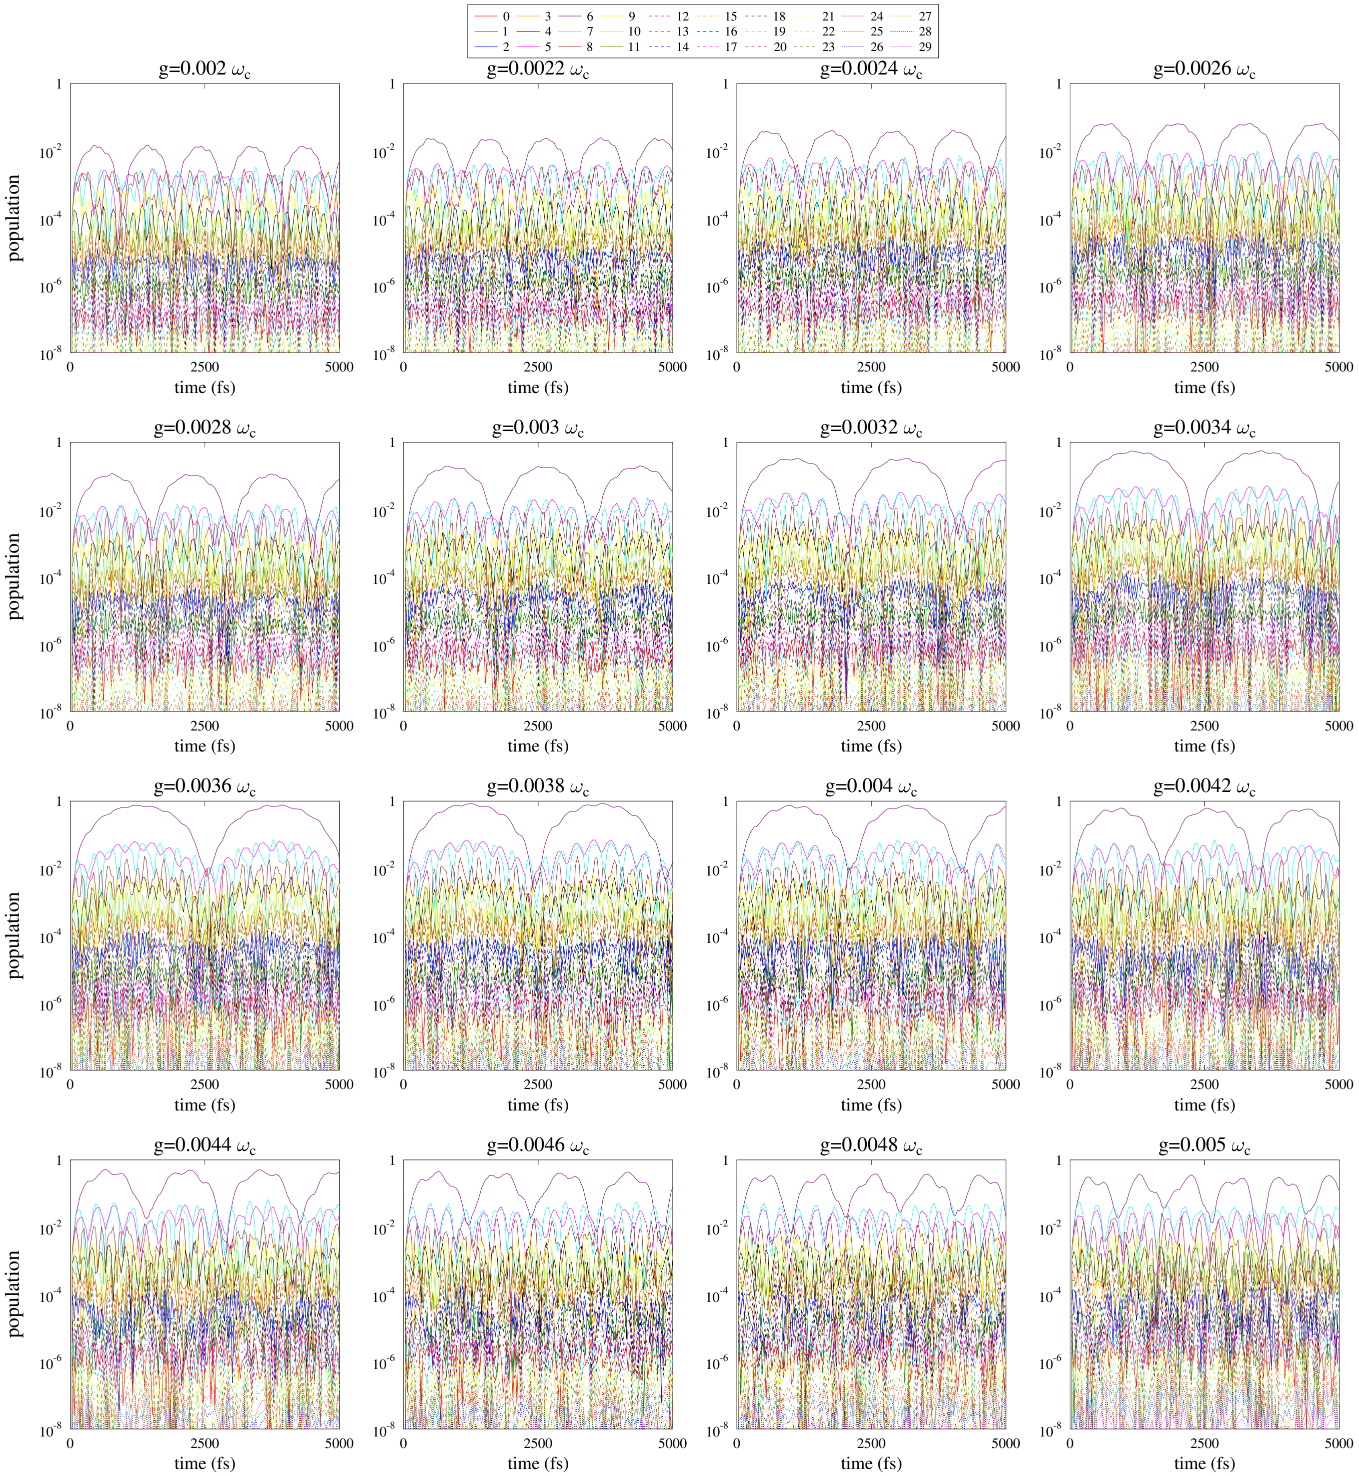


FIG. S3. Population dynamics of some relevant diabatic vibrational eigenstates for different g values.

## 5. Population dynamics for $\kappa = 0.0004$

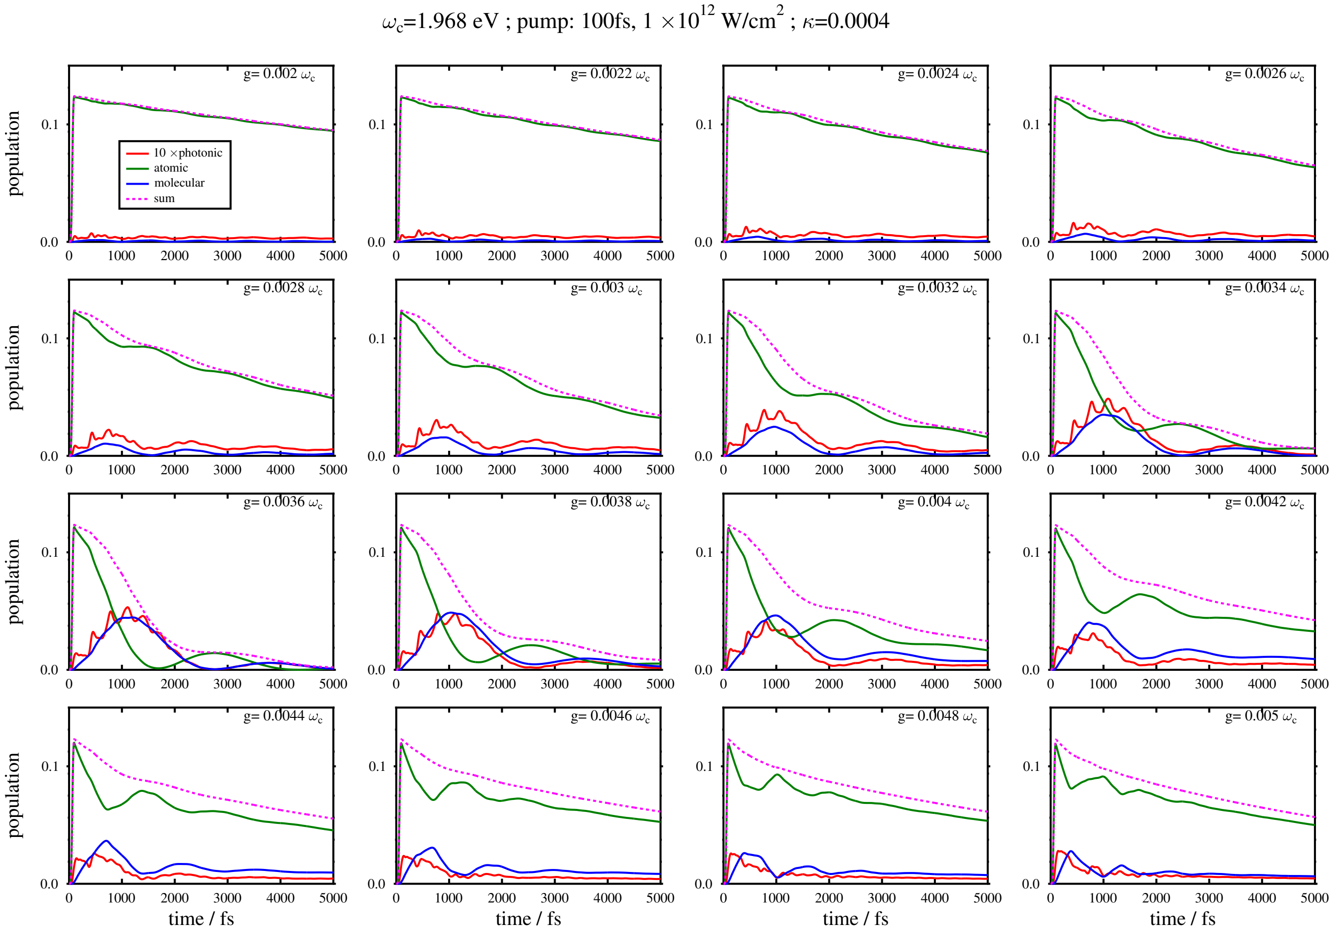


FIG. S4. The same as Fig.3 of the main text but for further cavity coupling strength values.

## 6. Population dynamics for $\kappa > 0.0004$

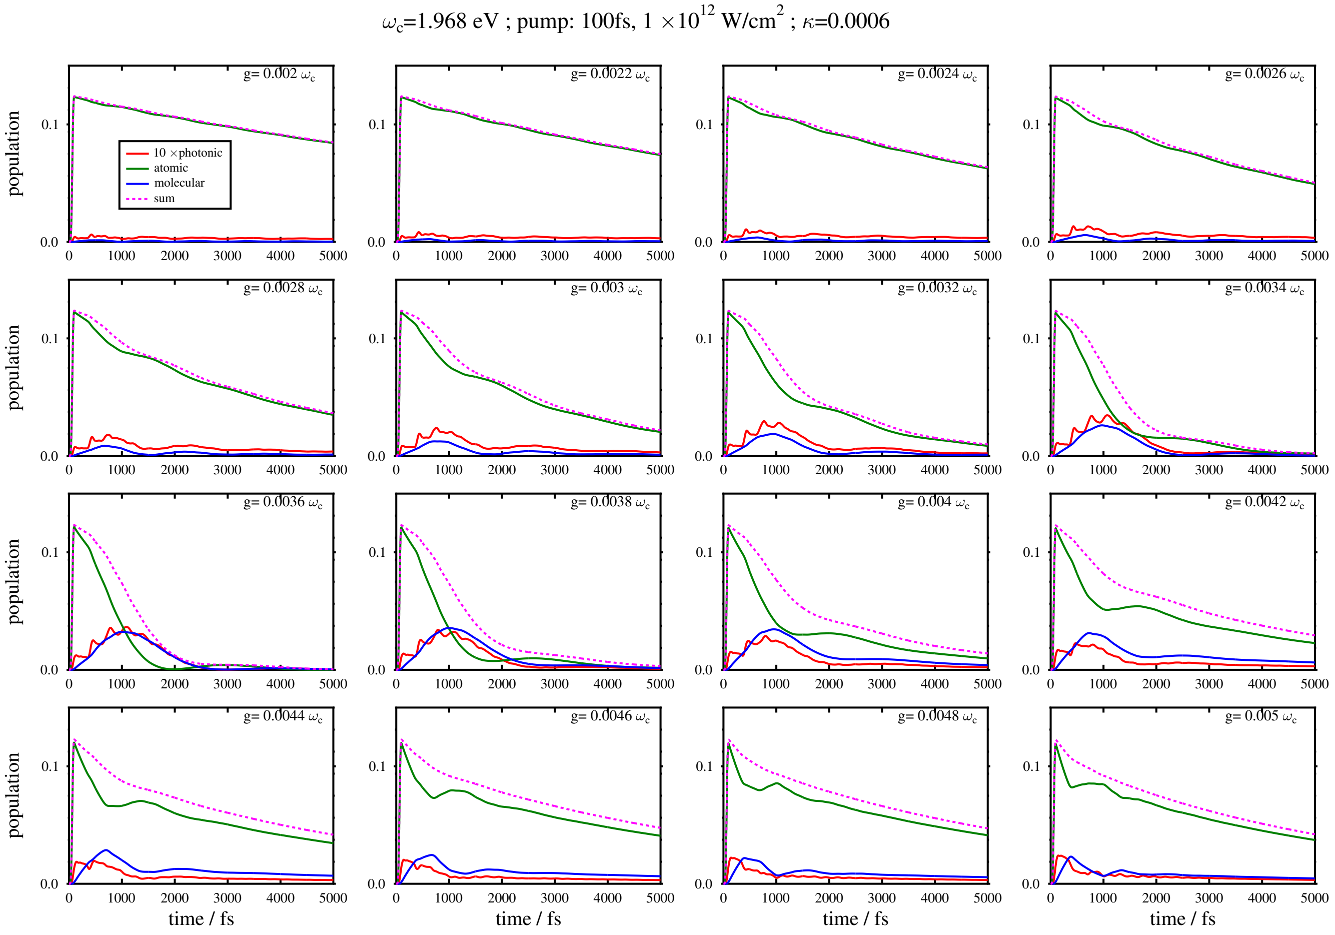


FIG. S5. The same as Fig.S4 above but for $\kappa = 0.0006$.

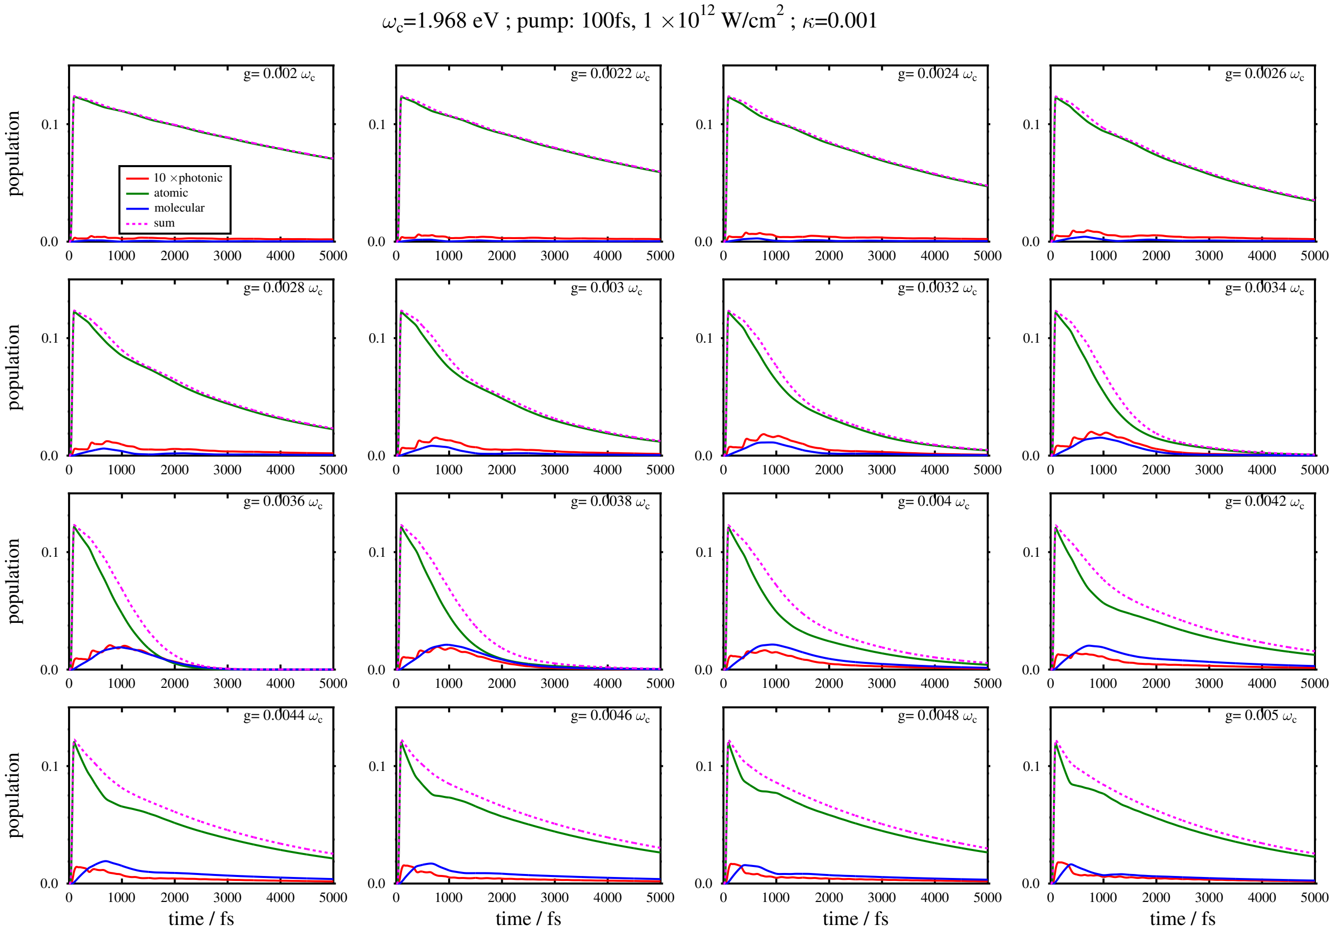


FIG. S6. The same as Fig.S4 above but for $\kappa = 0.001$.

[1] S. Magnier et al. J. Chem. Phys. 98 7113 (1993).
[2] W.T. Zemke et al. J. Mol. Spectrosc. 85 150 (1981).
[3] E. B. Saloman and Craig J. Sansonetti, Journal of Physical and Chemical Reference Data 33 1113 (2004).
[4] U. Manthe, H. D. Meyer, and L. S. Cederbaum, The Journal of Chemical Physics 97 3199 (1992).
[5] M. Beck, Physics Reports 324 1 (2000).
